# Supplementary material for: Efficient candidate screening under multiple tests and implications for fairness
Source: arXiv:1905.11361 source file (2019-05-27)
Supplement: Supplementary file 1 [file appendix.tex]

\paragraph*{Proofs from Section \ref{sec:oneGroup}}

\paragraph*{Proofs from Section \ref{sec:twoGroups}}

\paragraph*{Proofs from Section \ref{sec:gaussian}}

\paragraph*{Proofs from Section \ref{sec:gaussianTwoGroups}}

\paragraph*{Proofs from Section \ref{sec:unsupervised}}
